# Supplementary material for: A biological tissue-inspired tunable photonic fluid
Source: arXiv:1608.06334 ancillary file (2018-05-15)
Supplement: Supplementary file 1 [file SI_appendix_full.pdf]

# Supporting Information Appendix for *A tunable biological tissue-inspired photonic fluid*

Xinzhi Li, Amit Das, and Dapeng Bi
*Department of Physics,*
*Northeastern University, MA 02115, USA*

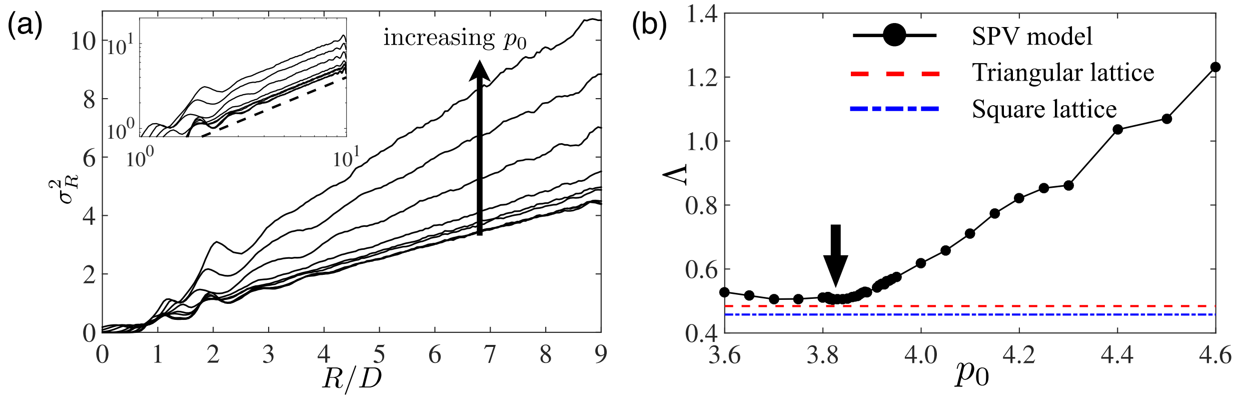


FIG. S1. **Unusual density fluctuations and hyperuniformity in the SPV model.** To characterize hyperuniformity, the number of cells contained within an observation window of radius $R$ and centered at $\boldsymbol{r}_0$ is calculated using $N_R = \int_{|\boldsymbol{r}-\boldsymbol{r}_0|<R} \rho(\boldsymbol{r}) d\boldsymbol{r}$, where $\rho(\boldsymbol{r}) = \sum_{i=1}^{M} \delta(\boldsymbol{r} - \boldsymbol{r}_i)$ is the number density. The cell number variance is then given by $\sigma_R^2 = \langle N_R^2 \rangle - \langle N_R \rangle^2$. Here $\langle ... \rangle$ averages over random observation windows and 200 SPV ground state configurations at each $p_0$. Configurations containing 400 cells are used for this calculation. **(a)** The cell number variation $\sigma_R^2$ is linearly proportional to the observation window size $R$ at various values of $p_0$. Different lines correspond to $p_0 = 3.25, 3.35, 3.813, 3.83, 3.87, 3.89, 3.93, 3.94, 4.5$. Inset shows the same data on a log − log plot, with the dashed line representing a slope of 1. **(b)** The constant of proportionality $\Lambda$ between $\sigma_R^2$ and $R$ is plotted as function of $p_0$. The black arrow indicates the location of the solid-fluid transition for tissues ($p_0 = 3.81$). Values corresponding to $\Lambda$ in crystalline structures [1] are given by the dashed lines.

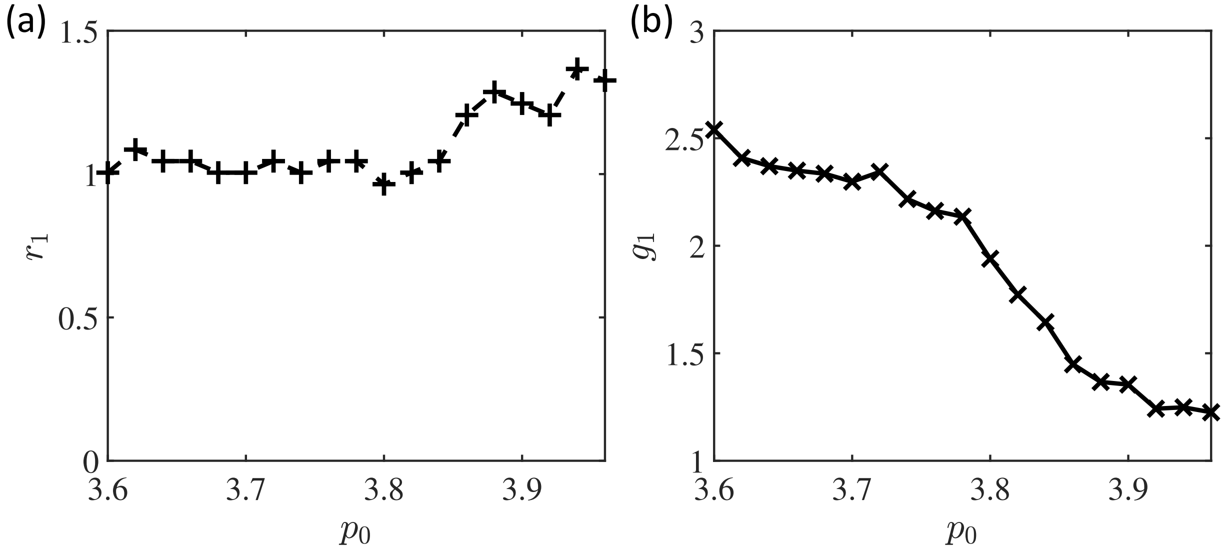


FIG. S2. **The properties of the pair correlation function $g(r)$ for various $p_0$ at zero temperature and $N = 256$.** **(a)** Position of the first peak of $g(r)$, defined as $r_1$ , has some deviation from $r = 1$ with the increasing of $p_0$. **(b)** Height of the first peak of $g(r)$, $g_1$, decreases monotonously when $p_0$ is increased, indicating the loss of short range order .

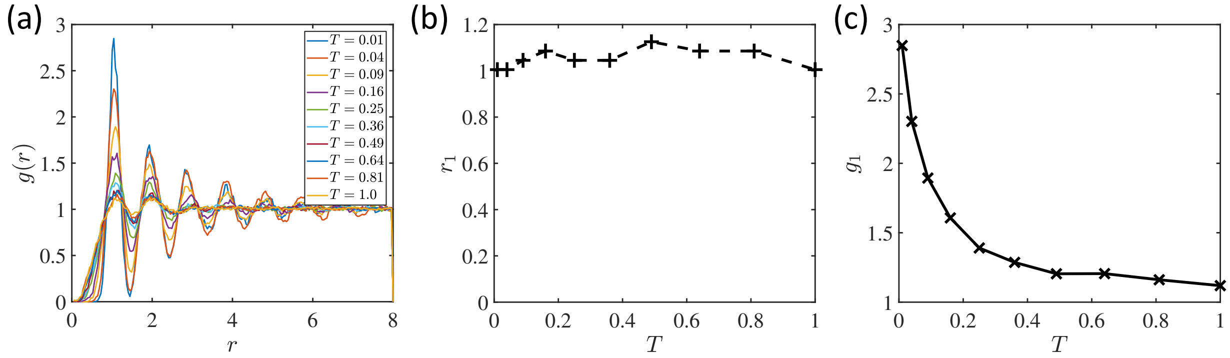


FIG. S3. **Pair correlation function** $g(r)$**.** (a) $g(r)$ at different temperatures $T$ and fixed $p_0 = 3.7$. To find a good measure that characterizes the structure of the system, we extract the position and height of the first peak of $g(r)$, shown in (b) and (c) respectively. We observe that $r_1$ shows very small difference, while $g_1$ decreases monotonously with increasing the temperature. At fixed $p_0$, when heating, the system is also losing short range order .

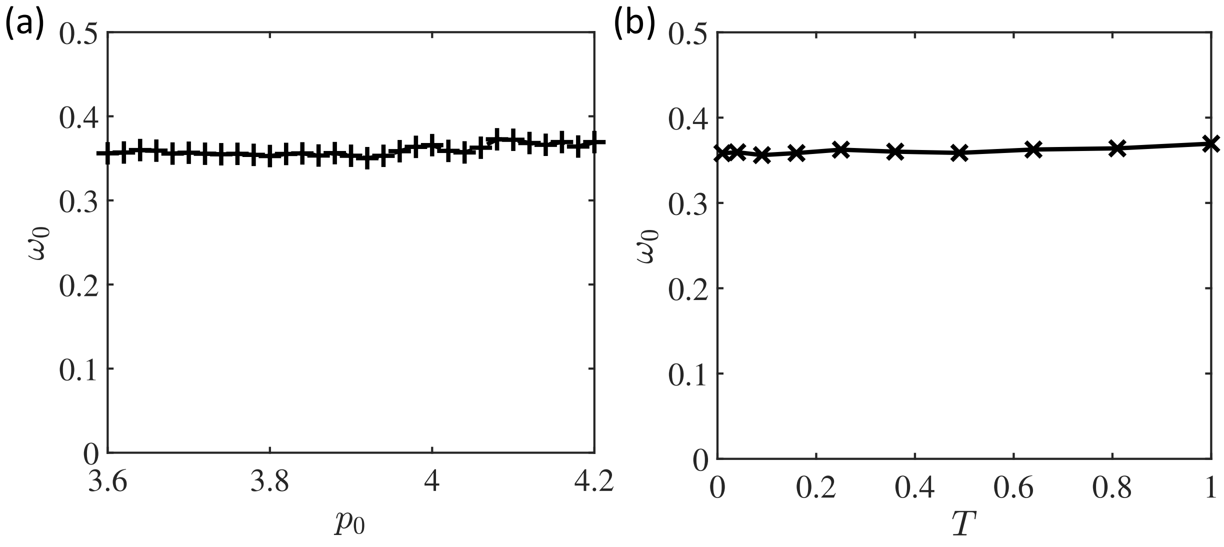


FIG. S4. (a) The midgap frequency of the PBG $\omega_0$ as function of $p_0$ at $T = 0$. (b) The midgap frequency of the PBG $\omega_0$ as function of $T$ at fixed $p_0 = 3.7$.

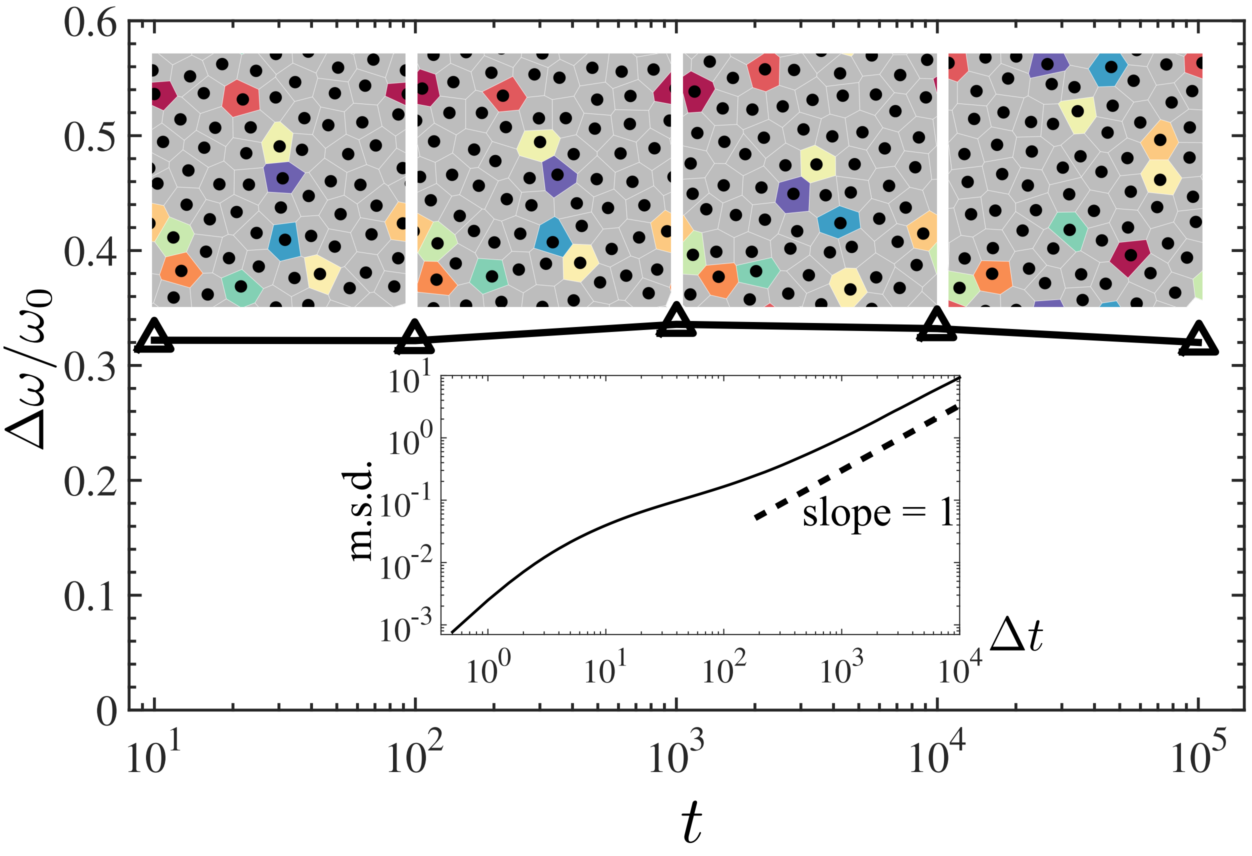


FIG. S5. **The photonic bandgap is robust under fluidization.** A finite temperature $T = 0.006$ is applied to a state at $p_0 = 3.82$. The TM gap-midgap ratio is plotted for different times spanning 4 decades in simulation time units. The material eventually fluidizes as shown by the mean squared displacement of cell centers (inset), with a structural relaxation time of $t \sim 10^3$. The snapshots are taken at $t = 10, 10^2, 10^3, 10^4$. Here, 10 cells are selected to show relative motion and rearrangements.

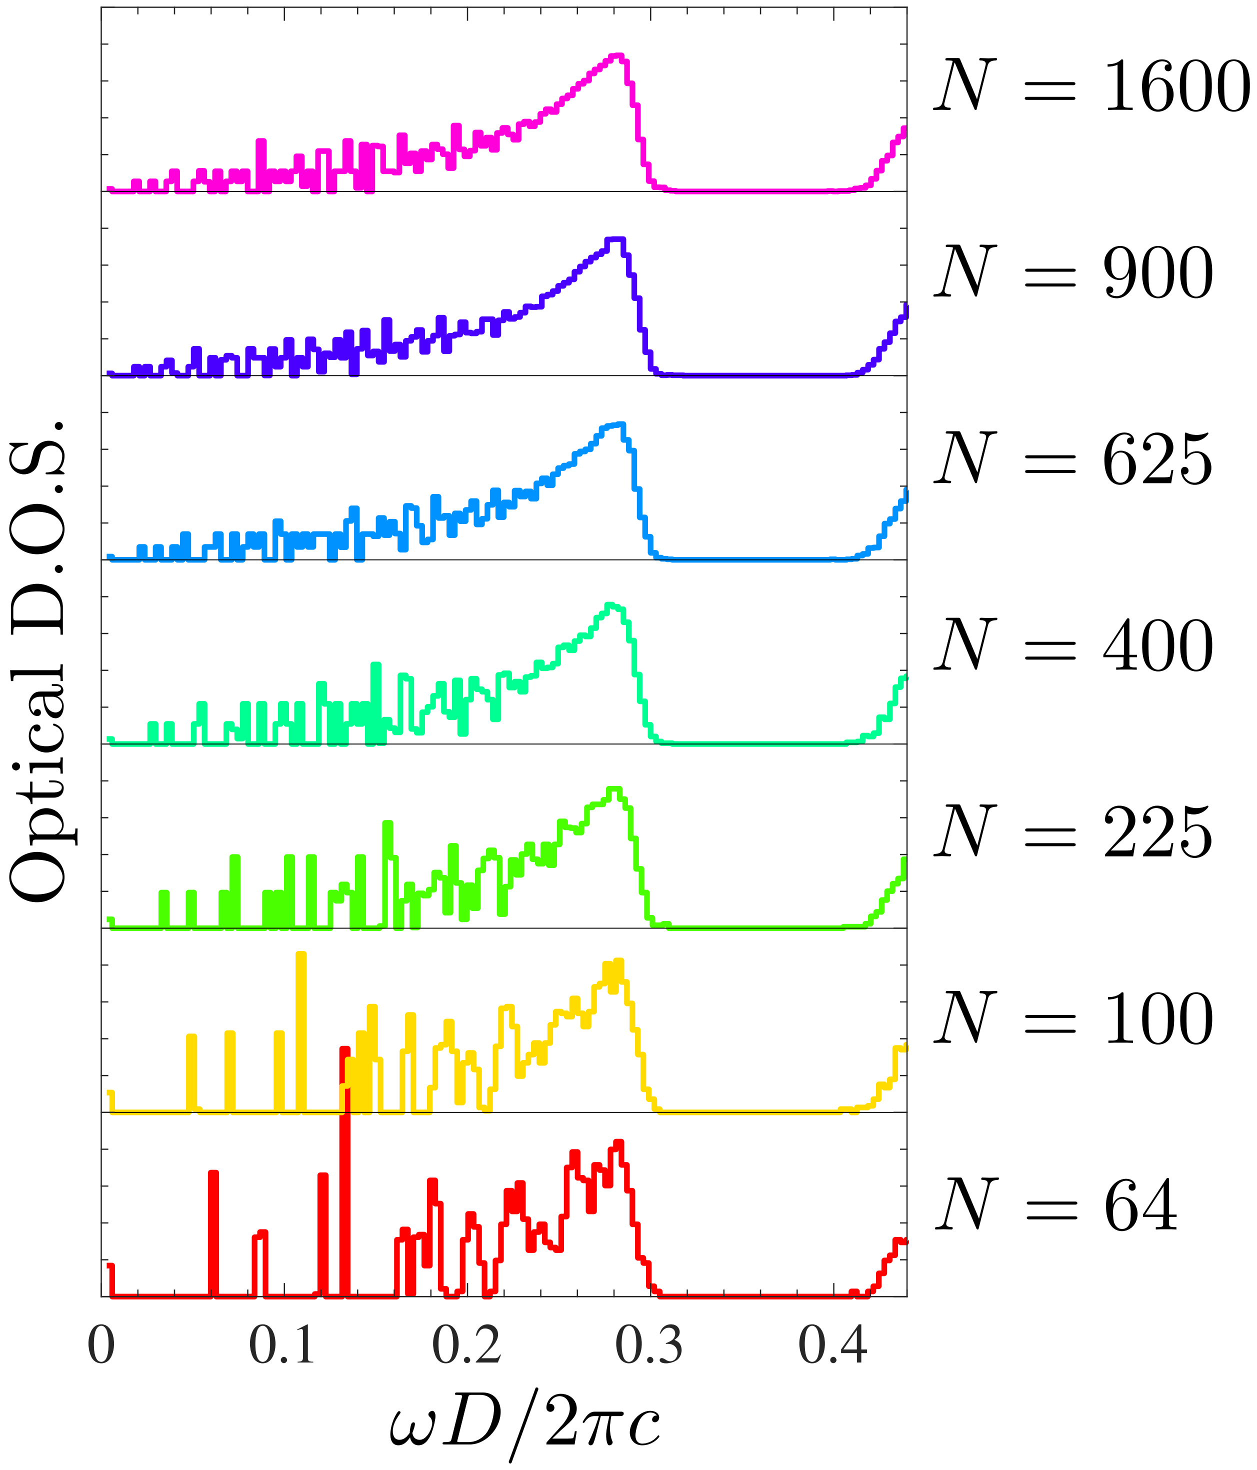


FIG. S6. **Finite-size effects on the photonic bandgap**. We measure the ODOS at $p_0 = 3.7$ for various system sizes ranging from $N = 64$ to 1600. At each system size, the ODOS was generated by tabulating TM frequencies along the $\boldsymbol{k}_{\parallel} = (0,0)$ and $\boldsymbol{k}_{\parallel} = (0.5,0.5)$ directions in reciprocal space for 10 randomly generated states. While low frequency modes may depend on the system size, the photonic bandgap, always located between mode number $N$ and $N+1$ spans a frequency range that does not change as function of $N$.

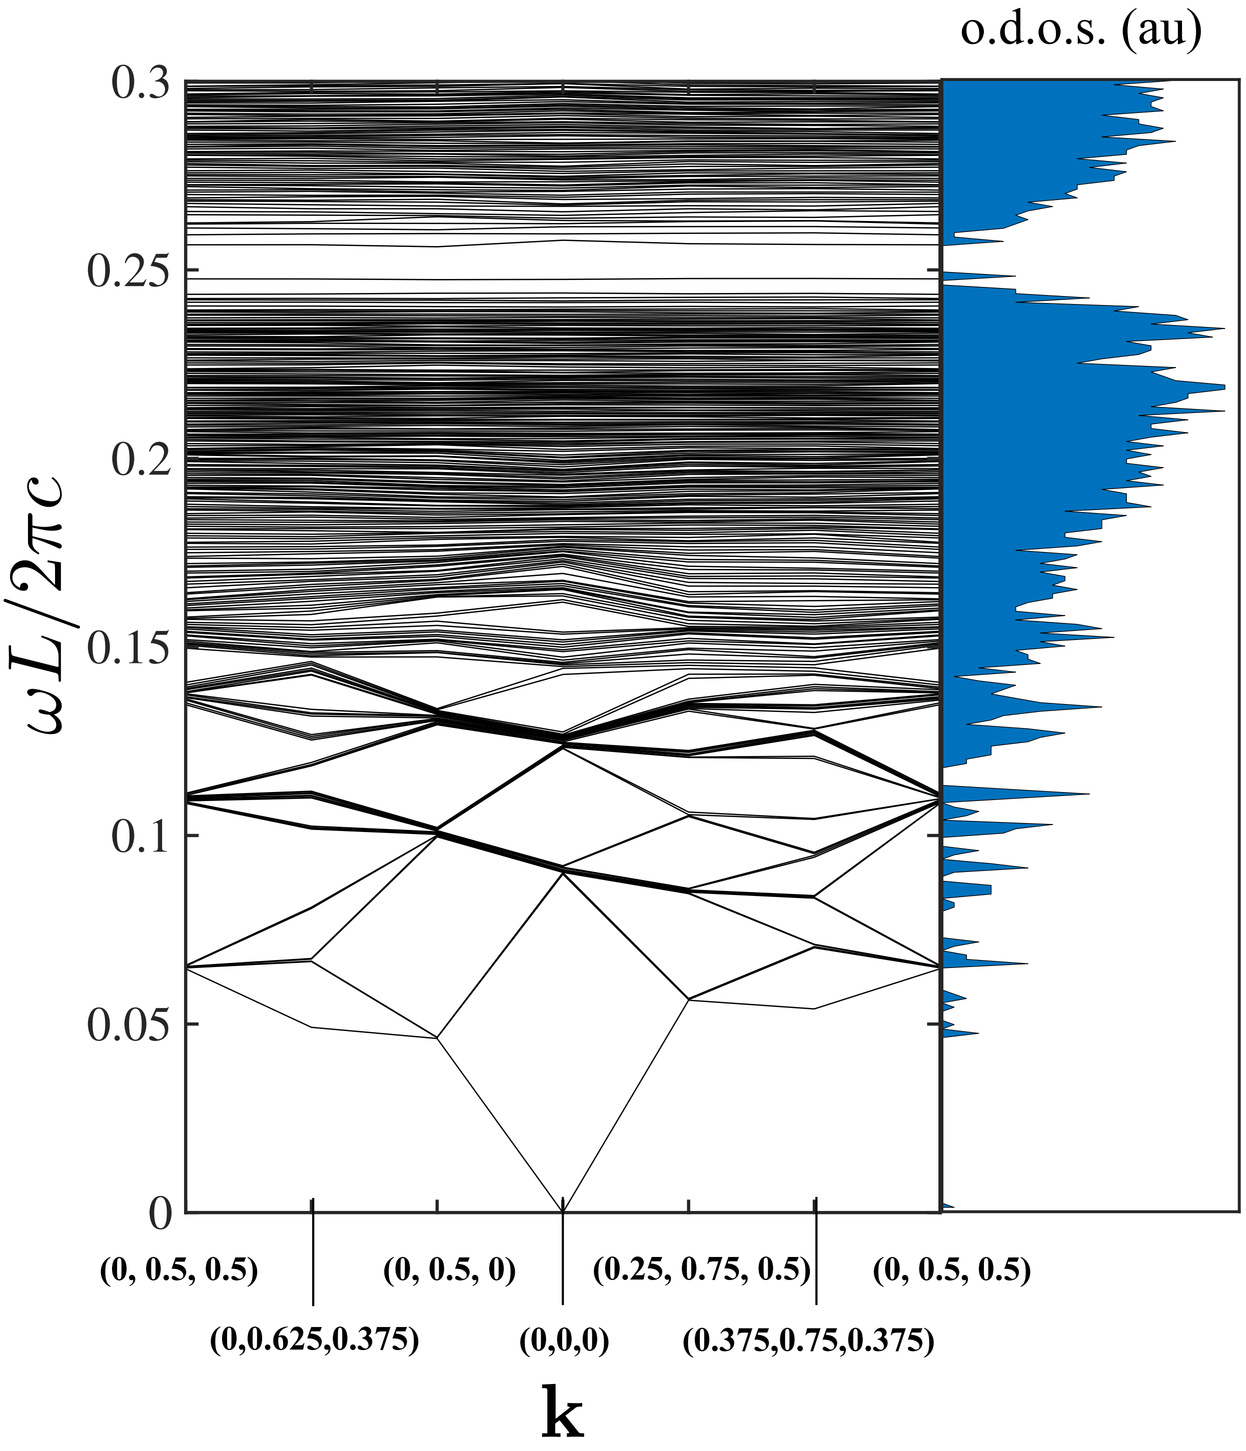


FIG. S7. The photonic band structure for the decorated 3D dielectric network designed using $s_0 = 5$ and $N = 40$ (illustrated in Fig. 5(c)). The eigenfrequencies are calculated along six reciprocal vectors. The optical density of states is calculated by tabulating all **k** results at each frequency and shown on the right-hand side.

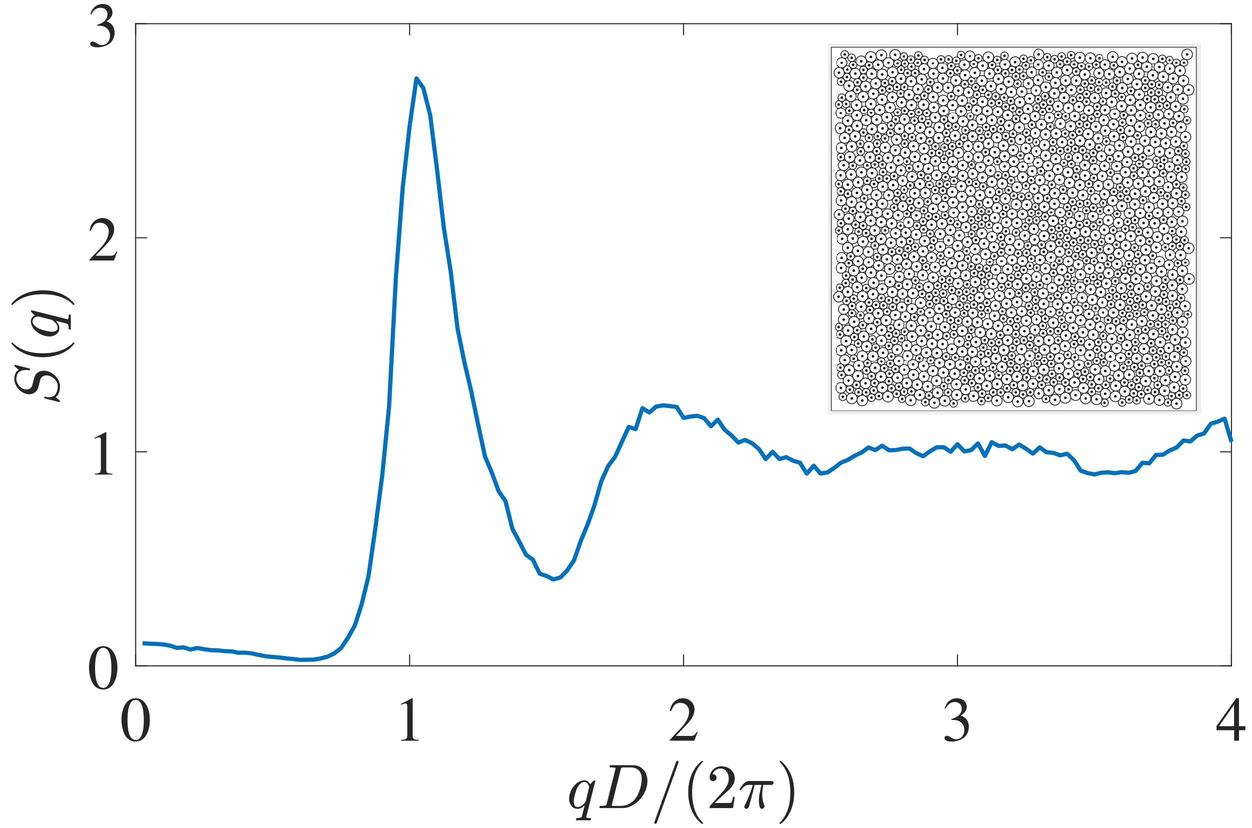


FIG. S8. In order to contrast and compare the hyperuniform patterns of the tissue model with patterns that are known to be non-hyperuniform, we generate 2D bi-dispersed jammed disk configurations with packing density $\phi = 0.86$, particle size ratio 1.4 at 50:50 mixture ratio[2]. To calculate $S(q)$, we use a system with $N = 1600$ particles and 10 different random configurations. $S(q)$ appears to be not hyperuniform.

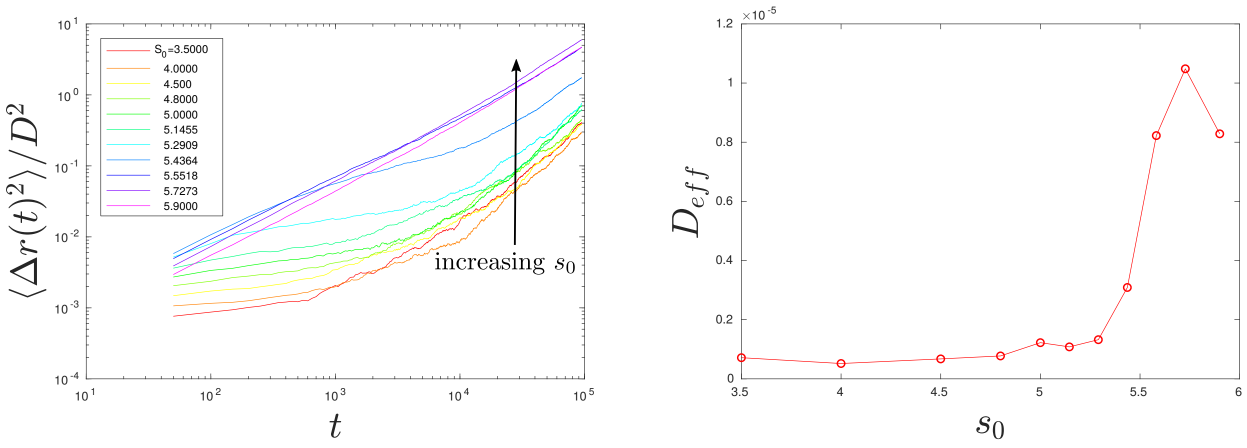


FIG. S9. Mean-square displacements $\langle \Delta r(t)^2 \rangle$ (left) and effective diffusivity $D_{eff}$ (right) of the cells in our simulations in three dimensions, at different $s_0$ values. The transition from soild-like to fluid-like behavior, around $s_0 = 5.4$, is quite prominent. Here, $D$ is the unit of length in the simulations defined as $D = V_0^{1/3}$, where $V_0$ is the preferred volume of the cells (also the average volume of the cells in our case). The effective diffusivity is calculated using Einstein's result: $D_{eff} = \langle \Delta r(t)^2 \rangle / 6t$ in the limit of large time $t$, or as in our simulations a large number of Monte-Carlo steps.

## I. MPB SAMPLE CODE

Sample MIT Photonic Bands (MPB) code for calculation of the TM eigenspectrum for a system of 16 dielectric rods is included below. The rod positions are based on the 2D SPV ground state at $p_0 = 3.7$. The code is based on the open source script from the MPB [3] website: https://mpb.readthedocs.io/en/latest/

```
(define-param eps 11.56) ; setting the dielectric constant of rods
(define GaAs (make dielectric (epsilon eps)))
(set! geometry-lattice (make lattice (size 4 4 no-size))) ; 2d super-cell
(define-param r 0.189) ; radius of the rods
(set! geometry ;  listing rod positions and geometry
(list
        ( make cylinder (material GaAs) (center 2.5588 0.906) (radius r) (height infinity) )
        ( make cylinder (material GaAs) (center 0.43963 1.3434)  (radius r) (height infinity) )
        ( make cylinder (material GaAs) (center 1.7984 0.02637)  (radius r) (height infinity) )
        ( make cylinder (material GaAs) (center 3.0053 0.10968)  (radius r) (height infinity) )
        ( make cylinder (material GaAs) (center 1.9216 2.7414)  (radius r) (height infinity) )
        ( make cylinder (material GaAs) (center 3.8384 0.68869)  (radius r) (height infinity) )
        ( make cylinder (material GaAs) (center 3.5071 1.624)  (radius r) (height infinity) )
        ( make cylinder (material GaAs) (center 1.312 2.1015) (radius r) (height infinity) )
        ( make cylinder (material GaAs) (center 3.2054 2.5391)  (radius r) (height infinity) )
        ( make cylinder (material GaAs) (center 0.96737 3.2383) (radius r) (height infinity) )
        ( make cylinder (material GaAs) (center 0.80395 0.2014) (radius r) (height infinity) )
        ( make cylinder (material GaAs) (center 2.252 1.8142)  (radius r) (height infinity) )
        ( make cylinder (material GaAs) (center 2.7571 3.3181)  (radius r) (height infinity) )
        ( make cylinder (material GaAs) (center 0.21168 2.4905) (radius r) (height infinity) )
        ( make cylinder (material GaAs) (center 1.5498 0.9486)  (radius r) (height infinity) )
        ( make cylinder (material GaAs) (center 3.9663 3.4222)  (radius r) (height infinity) )
))
(set! k-points (vector3 0 0 0)) ; define wave vector(s) for calculation of eigenspectrum
(set-param! resolution 16)  ; resolution sets the grid size for the calculation
(set-param! num-bands 18)  ; number of eigenfrequencies to calculate
(run-tm) ; begins calculation the eigenspectrum for the transverse-magnetic polarization
```


[1] Salvatore Torquato and Frank H. Stillinger, "Local density fluctuations, hyperuniformity, and order metrics," Phys. Rev. E **68**, 041113 (2003).

[2] Corey S. O'Hern, Leonardo E. Silbert, Andrea J. Liu, and Sidney R. Nagel, "Jamming at zero temperature and zero applied stress: The epitome of disorder," Phys. Rev. E **68**, 011306 (2003).

[3] Steven G. Johnson and J. D. Joannopoulos, "Block-iterative frequency-domain methods for maxwell's equations in a planewave basis," Opt. Express **8**, 173–190 (2001).
